# Supplementary material for: Synbit: Synthesizing Bidirectional Programs using Unidirectional Sketches
Source: arXiv:2108.13783 source file (2021-10-06)
Supplement: Supplementary file 1 [file appendix_experiments.tex]

\subsection{Details of Experiments of Section \ref{sec:experiment-comparative}}
% \subsubsection{Input and Output of Section \ref{sec:experiment-categorize}}
% \subsubsection{Input and Output of Section }

\subsubsection{$\var{double}$}
\paragraph{Input:}
\begin{codemath}
  \bb
  \var{go} :: \con{Nat} \to \con{Nat}\\
  \var{go}\A n = \CASE~n~\OF~
  \bbt
  \con{Z} & \to \con{Z}\\
  \con{S} \A n' & \to \CASE~n'~\OF~\{
  \bbt
  \con{S} \A n'' & \to ??\}
  \ee
  \ee\\\\
  \var{doubleP} :: \con{Nat} \to \con{Nat} \to \con{Nat}\\
  \var{doubleP} \A s \A v = go \A v\\\\
  \con{assert} \A (\var{doubleP} \A 1 \A 6 == 3)\\
  \con{assert} \A (\var{doubleP} \A 5 \A 4 == 2)
  \ee&&
\end{codemath}

\paragraph{Output:}
\begin{codemath}
  \bb
  ??_0= \con{S} \A (\var{go} \A \var{n''})
  \ee&&
\end{codemath}

\subsubsection{$\var{uncurryReplicate}$}
\paragraph{Input:}
\begin{codemath}
  \bb
  \var{length} :: \forall a. \con{List} \A a \to \con{Nat}\\
  \var{length}\A \langle a\rangle \A l = \CASE~l~\OF~
  \bbt
  \con{Nil} & \to \con{Z}\\
  \con{Cons} \A p & \to ??
  \ee\\\\
  \var{head} :: \forall a. \con{List} \A a \to a\\
  \var{head}\A \langle a\rangle \A l = \CASE~l~\OF~
  \{\bbt
  \con{Cons} \A p & \to ??
  \ee\}\\\\
  \var{uncurryReplicateP} :: \forall a. \langle a\rangle \A  (a,\con{Nat}) \to \con{List} \A a \to (a,\con{Nat})\\
  \var{uncurryReplicateP}\A \langle a\rangle \A s \A v = (\var{head} \A \langle a\rangle \A v,\var{length} \A \langle a\rangle \A v)\\\\
  \con{assert} \A (\var{uncurryReplicateP} \A \langle \con{Nat}\rangle \A (0, 2) \A [0,0,0] == (0, 3))\\
  \con{assert} \A (\var{uncurryReplicateP} \A \langle \con{Bool}\rangle \A (\con{True}, 3) \A [\con{False},\con{False}] == (\con{False}, 2))
  \ee&&
\end{codemath}

\paragraph{Output:}
\begin{codemath}
  \bb
  ??_0 = \con{S} \A (\var{length} \A \langle a\rangle \A (\#2.2 \A p))\\
  ??_1 = \#2.1 \A p
  \ee&&
\end{codemath}

\subsubsection{$\var{mapNot}$}
\paragraph{Input:}
\begin{codemath}
  \bb
  \var{not} :: \con{Bool} \A a \to \con{Bool}\\
  \var{not} \A b = \CASE~b~\OF~
  \bbt
  \con{True} & \to \con{False}\\
  \con{False} & \to \con{True}
  \ee\\
  \\
  \var{map} :: (\con{Bool} \to \con{Bool}) \to \con{List} \A \con{Bool} \to \con{List} \A \con{Bool}\\
  \var{map} \A f \A l = \CASE~l~\OF~
  \bbt
  \con{Nil} & \to \con{Nil} \A \langle \con{Bool} \rangle\\
  \con{Cons} \A p & \to ??
  \ee\\
  \\
  \var{mapNotP} :: \con{List} \A \con{Bool} \to \con{List} \A \con{Bool} \to \con{List} \A \con{Bool}\\
  \var{mapNotP} \A s \A v = \var{map} \A \var{not} \A v\\
  \\
  \con{assert} \A (\var{mapNotP} \A [\con{True},\con{False}] \A [\con{True},\con{True},\con{False}] == [\con{False},\con{False},\con{True}])\\
  \con{assert} \A (\var{mapNotP} \A [\con{True},\con{False}] \A [\con{True},\con{True},\con{False},\con{True}] == [\con{False},\con{False},\con{True},\con{False}])\\
  \con{assert} \A (\var{mapNotP} \A [\con{False},\con{True}] \A [\con{False}] == [\con{True}])
  \ee&&
\end{codemath}

\paragraph{Output:}
Timeout

\subsubsection{$\var{mapReplicate}$}
\paragraph{Input:}
\begin{codemath}
  \bb
  \var{map} :: \forall a \ b. (a \to b) \to \con{List} \A a \to \con{List} \A b\\
  \var{map}\A \langle a,b\rangle \A l = \CASE~l~\OF~
  \bbt
  \con{Nil} & \to \con{Nil} \A \langle b \rangle \\
  \con{Cons} \A p & \to ??
  \ee\\
  \\
  \var{length} :: \forall a. \con{List} \A a \to \con{Nat}\\
  \var{length}\A \langle a\rangle \A l = \CASE~l~\OF~
  \bbt
  \con{Nil} & \to \con{Z}\\
  \con{Cons} \A p & \to ??
  \ee\\
  \\
  \var{head} :: \forall a. \con{List} \A a \to a\\
  \var{head}\A \langle a\rangle \A l = \CASE~l~\OF~
  \{\bbt
  \con{Cons} \A p & \to ??
  \ee\}\\
  \\
  \var{replicateP} :: \forall a. \con{List} \A a \to (a,\con{Nat})\\
  \var{replicateP}\A \langle a\rangle \A v = (\var{head} \A \langle a\rangle \A v,\var{length} \A \langle a\rangle \A v)\\
  \\
  \var{mapReplicateP} :: \forall a. \A \con{List} \A (a,\con{Nat}) \to \con{List} \A (\con{List} \A a) \to \con{List} \A (a,\con{Nat})\\
  \var{mapReplicateP}\A \langle a\rangle \A s \A v = \var{map} \A \langle \con{List} \A a, (a,\con{Nat})\rangle \A (\var{replicateP} \A \langle a \rangle) \A v\\
  \\
  \con{assert} \A (\var{mapReplicateP} \A \langle \con{Nat}\rangle \A [(2,2)] \A [[1,1,1],[2],[3,3]] == [(1,3),(2,1),(3,2)])\\
  \con{assert} \A (\var{mapReplicateP} \A \langle \con{Nat}\rangle \A [(1,3),(2,1),(3,2)] \A [[2,2]] == [(2,2)]
  \ee&&
\end{codemath}

\paragraph{Output:}
Time out

\subsubsection{$\var{snoc}$}
\paragraph{Input:}
\begin{codemath}
  \bb
  \var{go} :: \forall a. \con{List} \A a \to (\con{List} \A a,a)\\
  \var{go}\A \langle a\rangle \A l =
  \LET~\con{Cons} \A p = l~\IN~
  \CASE~\#2.2 \A p~\OF~\bbt
  \con{Nil} & \to (\con{Nil}\A\langle a\rangle,\#2.1 \A p)\\
  \con{Cons} \A p & \to
  \bbt\LET~\bbt
  a:(\con{List} \A a,a)\\
  a = ??\ee\\
  \IN~??\ee\ee\\
  \\
  \var{snocP} :: \forall a. \A (\con{List} \A a,a) \to \con{List} \A a \to (\con{List} \A a,a)\\
  \var{snocP}\A \langle a\rangle \A s \A v = \var{go} \A \langle a \rangle \A v\\
  \\
  \con{assert} \A (\var{snocP} \A \langle \con{Nat}\rangle \A ([1, 2, 3], 4) \A [1, 2, 3] == ([1, 2], 3))\\
  \con{assert} \A (\var{snocP} \A \langle \con{Nat}\rangle \A ([1, 2, 3], 4) \A [1, 2, 3, 4, 5, 6] == ([1, 2, 3, 4, 5], 6))
  \ee&&
\end{codemath}

\paragraph{Output:}
No solutions.

\subsubsection{$\var{length}$ and $\var{lengthTail}$}
\paragraph{Input:}
\begin{codemath}
  \bb
  \var{replicate} :: \forall a. a \to \con{Nat} \to \con{List}\A a\\
  \var{replicate}\A \langle a\rangle \A x \A n = \CASE~n~\OF~
  \bbt
  \con{Z} & \to \con{Nil} \A \langle a\rangle\\
  \con{S} \A n' & \to ??
  \ee\\\\
  \var{take} :: \forall a. \con{Nat} \to \con{List}\A a\to \con{List}\A a\\
  \var{take}\A \langle a\rangle \A x \A n = \CASE~n~\OF~
  \bbt
  \con{Z} & \to \con{Nil} \A \langle a\rangle\\
  \con{S} \A n' & \to \CASE~l~\OF~
  \bbt
  \con{Nil} & \to \con{Nil} \A \langle a\rangle\\
  \con{Cons} \A p & \to ??
  \ee
  \ee\\\\
  \var{append} :: \forall a. \con{List}\A a\to \con{List}\A a\to \con{List}\A a\\
  \var{append}\A \langle a\rangle \A l_1 \A l_2 = \CASE~l_1~\OF~
  \bbt
  \con{Nil} & \to l_2\\
  \con{Cons} \A p & \to ??
  \ee\\\\
  \var{go} :: \forall a. \con{List} \A a \to (\con{List} \A a,a)\\
  \var{go}\A \langle a\rangle \A l =
  \LET~\con{Cons} \A p = l~\IN~
  \CASE~\#2.2 \A p~\OF~\bbt
  \con{Nil} & \to (\con{Nil}\A\langle a\rangle,\#2.1 \A p)\\
  \con{Cons} \A p & \to
  \bbt\LET~\bbt
  a:(\con{List} \A a,a)\\
  a = ??\ee\\
  \IN~??\ee\ee\\
  \\
  \var{lengthP} :: \con{List}\A \con{Nat}\to\con{Nat}\to \con{List}\A \con{Nat}\\
  \var{lengthP}\A s \A v = \var{take} \A \langle \con{Nat} \rangle \A v \A (\var{append}\A \langle \con{Nat} \rangle \A s\A (\var{replicate} \A \langle \con{Nat} \rangle \A 0 \A v))\\
  \\
  \con{assert} \A (\var{lengthP} \A \langle \con{Nat}\rangle \A [1,2] \A 4 == [1,2,0,0]\\
  \con{assert} \A (\var{lengthP} \A \langle \con{Nat}\rangle \A [2,0] \A 1 == [2])\\
  \con{assert} \A (\var{lengthP} \A \langle \con{Nat}\rangle \A [1,2] \A 5 == [1,2,0,0,0]
  \ee&&
\end{codemath}

\paragraph{Output:}
Time out

\subsubsection{$\var{reverse}$}
\paragraph{Input:}
\begin{codemath}
  \bb
  \var{revAppend} :: \forall a. \con{List}\A a\to \con{List}\A a\to \con{List}\A a\\
  \var{revAppend}\A \langle a\rangle \A \var{acc} \A l = \CASE~l~\OF~
  \bbt
  \con{Nil} & \to \var{acc}\\
  \con{Cons} \A p & \to ??
  \ee\\\\
  \var{reverseP} :: \forall a. \con{List}\A a\to \con{List}\A a\to \con{List}\A a\\
  \var{reverseP}\A \langle a\rangle\A s \A v = \var{revAppend} \A \langle a \rangle \A (\con{Nil} \A \langle a\rangle) \A v\\
  \\
  \con{assert} \A (\var{reverseP} \A \langle \con{Bool}\rangle \A [\con{True},\con{True}] \A [\con{False},\con{True},\con{True}] == [\con{True},\con{False},\con{False}]\\
  \con{assert} \A (\var{reverseP} \A \langle \con{Nat}\rangle \A [1,2,3,4] \A [6,5] == [5,6])
  \ee&&
\end{codemath}

\paragraph{Output:}
No solutions.

\subsubsection{$\var{add}$}
\paragraph{Input:}
\begin{codemath}
  \bb
  \var{addP} :: (\con{Nat},\con{Nat}) \to \con{Nat} \to (\con{Nat},\con{Nat})\\
  \var{addP}\A s \A v = \CASE~\#2.1\A s~\OF~
  \bbt
  \con{Z} & \to (\con{Z},v)\\
  \con{S} \A s' & \to \CASE~v~\OF~
  \bbt
  \con{Z} & \to (\con{Z},\con{Z})\\
  \con{S} \A v' & \to ??
  \ee
  \ee\\\\
  \con{assert} \A (\var{addP} \A (2,3) \A 7 == (2,5))\\
  \con{assert} \A (\var{addP} \A (2,3) \A 1 == (1,0))\\
  \con{assert} \A (\var{addP} \A (3,3) \A 4 == (3,1))
  \ee&&
\end{codemath}

\paragraph{Output:}
No solutions.

\subsubsection{$\var{professor}$}
\paragraph{Input:}
\begin{codemath}
  \bb
  \con{type} \A \con{PS} = \con{Professor} \A \con{Nat} \mid \con{Student} \A \con{Nat}\\\\
  \var{professorP} :: \con{List}\A \con{PS}\to \con{List}\A \con{Nat}\to \con{List}\A \con{PS}\\
  \var{professorP} \A s \A v = \CASE~s~\OF~
  \bbt
  \con{Nil} & \to
  \CASE~v~\OF~
  \bbt
  \con{Nil} \to \con{Nil} \A \langle \con{PS} \rangle\\
  \con{Cons} \A \var{pv} \to ??
  \ee
  \\
  \con{Cons} \A \var{ps} & \to \CASE~(\#2.1 \A \var{ps})~\OF~
  \bbt
  \con{Professor} \A \var{ids} \to
  \CASE~v~\OF~
  \bbt
  \con{Nil} \to ??\\
  \con{Cons} \A \var{pv} \to ??
  \ee
  \\
  \con{Student} \A \var{id} \to ??
  \ee
  \ee\\\\
  \con{assert} \A (\bbt \var{professorP} \A [\con{Student} \A 11, \con{Student} \A 12, \con{Professor} \A 21, \con{Student} \A 13, \con{Professor} \A 22]\A [31,32,33]\\
  = \A [\con{Student} \A 11, \con{Student} \A 12, \con{Professor} \A 31, \con{Student} \A 13, \con{Professor} \A 32, \con{Professor} \A 33])\ee\\
  \con{assert} \A (\bbt \var{professorP} \A [\con{Student} \A 11, \con{Student} \A 12, \con{Professor} \A 21, \con{Student} \A 13, \con{Professor} \A 22]\A [31]\\
  = \A [\con{Student} \A 11, \con{Student} \A 12, \con{Professor} \A 31, \con{Student} \A 13])\ee\\
  \con{assert} \A (\bbt \var{professorP} \A [\con{Student} \A 11, \con{Student} \A 12, \con{Professor} \A 21, \con{Student} \A 13, \con{Professor} \A 22]\A [31,32,33,34]\\
  = \A [\con{Student} \A 11, \con{Student} \A 12, \con{Professor} \A 31, \con{Student} \A 13, \con{Professor} \A 32, \con{Professor} \A 33, \con{Professor} \A 34])\ee\\
  \ee&&
\end{codemath}

\paragraph{Output:}
No solutions.

\subsubsection{$\var{splitBy0}$ ($\var{lines}$)}
\paragraph{Input:}
\begin{codemath}
  \bb
  \var{append} :: \forall a. \con{List}\A a\to \con{List}\A a\to \con{List}\A a\\
  \var{append}\A \langle a\rangle \A l_1 \A l_2 = \CASE~l_1~\OF~
  \bbt
  \con{Nil} & \to l_2\\
  \con{Cons} \A p & \to ??
  \ee\\\\
  \var{isLast0} :: \con{List}\A \con{Nat}\to \con{Bool}\\
  \var{isLast0}\A l = \CASE~l_1~\OF~
  \bbt
  \con{Nil} & \to \con{False}\\
  \con{Cons} \A p & \to \CASE~\#2.2 \A p~\OF~
  \bbt
  \con{Nil} & \to \CASE~\#2.1 \A p~\OF~\bbt
  \con{Z} \to \con{True}\\
  \con{S} \A n \to \con{False}\\
  \ee\\
  \con{Cons} \A p_2 & \to ??
  \ee\ee\\\\
  \var{splitBy0} :: \con{List}\A \con{Nat} \to \con{List} \A (\con{List} \A \con{Nat}) \to \con{List}\A \con{Nat}\\
  \var{splitBy0} \A s \A v = \CASE~v~\OF~
  \bbt
  \con{Nil} & \to \CASE~\var{isLast0} \A s ~\OF~
  \bbt
  \con{True} & \to \con{Cons} \A \langle\con{Nat}\rangle \A (\con{Z},\con{Nil} \A \langle\con{Nat}\rangle)\\
  \con{False} & \to \con{Nil} \A \langle\con{Nat}\rangle
  \ee\\
  \con{Cons} \A p & \to ??
  \ee\\\\
  \con{assert} \A (\var{splitBy0} \A [1,1,0,2,2,0,3,3] \A [[1,1], [2,2]] == [1,1,2,2]\\
  \con{assert} \A (\var{splitBy0} \A [1,1] \A [[1,1], [2,2]] == [1,1,2,2]\\
  \con{assert} \A (\var{splitBy0} \A [1,1,0] \A [[1,1], [2,2]] == [1,1,2,2,0]
  \ee&&
\end{codemath}

\paragraph{Output:}
Time out

\subsubsection{$\var{lookup}$}
\paragraph{Input:}
\begin{codemath}
  \bb
  \var{eq} :: \con{Nat} \to \con{Nat} \to \con{Bool}\\
  \var{eq}\A m \A n = \CASE~m~\OF~
  \bbt
  \con{Z} & \to \CASE~n~\OF~
  \bbt
  \con{Z} & \to \con{True}\\
  \con{S} \A n' & \to \con{False}
  \ee\\
  \con{S} \A m' & \to \CASE~n~\OF~
  \bbt
  \con{Z} & \to \con{False}\\
  \con{S} \A n' & \to ??
  \ee
  \ee\\\\
  \var{go} :: \con{List}\A (\con{Nat},\con{Nat}) \to \con{Nat} \to \con{Nat}\\
  \var{go} \A l \A v = \CASE~l~\OF~
  \bbt
  \con{Cons} \A p & \to \CASE~\var{eq} \A (\#2.2 \A (\#2.1 p)) \A v~\OF~
  \bbt
  \con{True} & \to \#2.1 \A (\#2.1 \A p)\\
  \con{False} & \to ??
  \ee\ee\\\\
  \var{lookupP} :: (\con{List}\A (\con{Nat},\con{Nat}),\con{Nat}) \to \con{Nat} \to (\con{List}\A (\con{Nat},\con{Nat}),\con{Nat})\\
  \var{lookupP} \A s \A v = (\#2.1 \ s, \var{go} \A (\#2.1 \A s) \A v)\\\\
  \con{assert} \A (\var{lookupP} \A ([(1,10), (2,200), (3,330)],2) \A 10 == (\var{lookupP} \A ([(1,10), (2,200), (3,330)],1)\\
  \con{assert} \A (\var{lookupP} \A ([(1,10), (2,200), (3,33)],2) \A 33 == (\var{lookupP} \A ([(1,10), (2,200), (3,33)],3)\\
  \con{assert} \A (\var{lookupP} \A ([(1,10), (2,200), (3,33)],2) \A 200 == (\var{lookupP} \A ([(1,10), (2,200), (3,33)],2)\\
  \ee&&
\end{codemath}

\paragraph{Output:}
\begin{codemath}
  \bb
  ??_0 = \var{eq} \A m' \A n'\\
  ??_1 = \var{go} \A (\#2.2 \A p) \A v
  \ee &&
\end{codemath}
